# Supplementary material for: Monochromatization of Electron Beams with Spatially and Temporally Modulated Optical Fields
Source: arXiv:2411.06814 source file (2025-01-07)
Supplement: Supplementary file 1 [file CM_SI.pdf]

# Supplemental Material: Monochromatization of electron beams with spatially and temporally modulated optical fields

Neli Laštovičková Streshkova,[1,*] Petr Koutenský,[1] Tomáš Novotný,[2] and Martin Kozák[1]

[1]*Department of Chemical Physics and Optics, Faculty of Mathematics and Physics, Charles University, Ke Karlovu 3, Prague CZ-12116, Czech Republic.*

[2]*Department of Condensed Matter Physics, Faculty of Mathematics and Physics, Charles University, Ke Karlovu 5, Prague CZ-12116, Czech Republic.*

(Dated: November 11, 2024)

## I. PROPOSED GEOMETRY AND PHASE MATCHING

The most common approaches how to realize the inelastic interaction between electrons and photons in vacuum are scattering on an optical beat wave, scattering on semi-infinite fields or scattering on optical near-fields. These methods all yield similar results for the modulation of longitudinal momentum of electrons, although the character of the transverse momentum modulation is different in general. In the paper we study the modulation of the kinetic energy and longitudinal momentum of the electrons via the interaction with ponderomotive potential of a chirped optical beat wave in non-relativistic regime (both the electron velocity and the normalized electric fields used in the calculations are small enough that the relativistic effects are negligible).

An optical beat wave, whose frequency can be expressed as $\omega = \omega_1 - \omega_2$, is formed by two optical fields with frequencies $\omega_i$ ($i = 1, 2$) which intersect at angles $\alpha_i$ with respect to the electron beam propagation axis $z_{\text{lab}}$, see Fig. S1. To reach efficient energy and momentum exchange between the electrons and the optical wave, both the energy and momentum conservation laws have to be fulfilled. The latter is referred to as a phase matching condition. In our geometry of choice the phase matching condition is given by the equation [S1]

$$\frac{c}{v_0} = \frac{\omega_1 \cos(\alpha_1) - \omega_2 \cos(\alpha_2)}{\omega_1 - \omega_2}, \tag{S1}$$

where $c$ is the speed of light, $v_0$ is the mean group velocity of the electron wave packet and and $\alpha_1$ and $\alpha_2$ are the angles of incidence of the two laser beams with respect to the electron beam. Although in general the instantaneous electron group velocity $v$ of the chirped electron pulse changes with respect to time, we can assume that the interaction time is short (in our case $v_0 \approx 1/3c$, interaction region $\approx \mu\text{m}$), that the interaction itself is weak (electric field amplitude of $\approx 2 \cdot 10^9\ \text{V} \cdot \text{m}^{-1}$) and both the chirp and the shift of the electron wave packet's kinetic energy due to the interaction with light is small compared to its initial energy (electrons accelerated to $>$ keV energies, $\Delta E \approx 5$ eV). The change of the electron velocity during the interaction thus can be neglected for the description of the electron trajectory during the interaction with light fields.

For given frequencies $\omega_1$, $\omega_2$, the equation (S1) can be fulfilled for different combinations of the angles $\alpha_1$, $\alpha_2$. Additionally we assume zero net transverse momentum change of the electrons [S1]

$$\omega_1 \sin(\alpha_1) = \omega_2 \sin(\alpha_2). \tag{S2}$$

By combining Eqs. (S1) and (S2) we obtain the values $\omega_1$, $\omega_2$, $\alpha_1$ and $\alpha_2$ that satisfy both constrains. The solution of Eqs. (S1) and (S2) is straightforward when $\omega_1$ and $\omega_2$ are constants. However, for the electron chirp compensation we require time dependent frequencies and therefore it is needed to fulfill Eqs. (1) and (2) in the center of the interaction region for the instantaneous values of $\omega_1$ and $\omega_2$.

As stated in the article, we conduct the calculations in the free electron rest frame for subrelativistic velocity $v_0$, where $t = t_{\text{lab}}$ and $z = z_{\text{lab}} - v_0 t$. The optical beams propagating under angle $\alpha_i$ in the $yz$ plane are characterized by the wave argument

$$\xi_i(\alpha_i, t, y, z_{\text{lab}}) = t - \frac{\mathbf{k}_i(\alpha_i) \cdot \mathbf{r}_{\text{lab}}}{\omega_i} = t - \frac{y \sin(\alpha_i) + z_{\text{lab}} \cos(\alpha_i)}{c}, \tag{S3}$$

and in the electron rest frame

$$\xi_i(\alpha_i, t, y, z) = t - \frac{y \sin(\alpha_i) + (z + v_0 t) \cos(\alpha_i)}{c}. \tag{S4}$$

* neli.streshkova@matfyz.cuni.cz

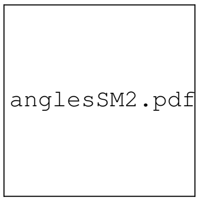


FIG. S1. Geometry of the optical beam intersection. The wave arguments $\xi_i = t - \mathbf{k}_i \cdot \mathbf{r}_{\text{lab}}/\omega_i$ describe the plane wave propagation arguments for each of the two beams at given time and angle of propagation in the laboratory frame. Different frequency components $\omega_i(\xi_i)$ of the optical wave are incident on the interaction region at different times and at different angles $\alpha_i(\xi_1, \xi_2)$.

The term $z\cos(\alpha_i)$ is the component of the electric field along the path of the electron and the term $y\sin(\alpha_i)$ is the component perpendicular to it. A quasi-monochromatic plane wave with constant frequency $\omega_i$ is described by $e^{-i\omega_i\xi_i}$. To satisfy the vacuum wave equation, we describe the chirped plane wave propagating in time and space by adding quadratic dependence on $\xi$ and obtaining $\exp\big[-i\omega_{0,i}\xi_i - ia_i\xi_i^2\big]$. We denote the central carrier frequency by $\omega_{0,i}$ and the chirp by $a_i$. The instantaneous frequency $\omega_i(\xi)$ reads

$$\omega_i(\xi_i) = \omega_{0,i} + 2a_i\xi_i. \tag{S5}$$

In the given geometry, $\omega_i$ are functions of the wave arguments $\xi_i$, therefore the angles $\alpha_i(\omega_1, \omega_2)$, which solve Eqs. (S1) and (S2) are in general also functions of $\xi_i$. By definition $\xi_i$ is dependent on $\alpha_i$. While the spatio-temporal chirp of the optical pulses leads to a nonlinear problem, we can find a sufficient region of overlap around $t = 0$, $z = 0$ where we can approximate this dependence by a linear function.

### A. Exact solution

Without loss of generality we assume phase matching only on the $z$ axis, which is reasonable for narrow electron beams. The angles required for the phase matching can be calculated for each $\xi_i$ on the $z$ axis directly from the geometry.

We iteratively solve the set of equations [S1] evaluated $\forall\xi_i(\alpha_i, t, 0, z)$

$$\alpha_1(\xi_1, \xi_2) = \arcsin\left(\frac{\omega_2(\xi_2)}{\omega_1(\xi_1)}\sin(\alpha_2(\xi_1, \xi_2))\right), \tag{S6}$$

$$u(\xi_1, \xi_2) = mc\sqrt{\left(\hbar\frac{\omega_1(\xi_1) - \omega_2(\xi_2)}{m_0c^2} + \gamma\right) - 1}\,, \tag{S7}$$

$$\alpha_2(\xi_1, \xi_2) = \arccos\left(\frac{\hbar^2(\omega_1(\xi_1) - \omega_2(\xi_2))(\omega_1(\xi_1) + \omega_2(\xi_2)) - c^2(u - \gamma m_0v_0)^2}{2\hbar c\omega_2(\xi_2)(u - \gamma m_0v_0)}\right), \tag{S8}$$

where $\gamma = (1 - v_0^2/c^2)^{-1/2}$ is the relativistic Lorentz factor and $m_0$ is the rest mass of the electron. In the first step we evaluate $\alpha_{0,1}$ and $\alpha_{0,2}$ from Eqs. (S6)-(S8) for the constant central frequencies $\omega_{0,1}$ and $\omega_{0,2}$. In the next step we evaluate $\alpha_i(\xi_i(\alpha_{0,i}))$ by plugging $\omega_i(\xi_i) = \omega_{0,i} + 2a_i\xi_i(\alpha_{0,i})$ into Eqs. (S6)-(S8). This cycle is iterated until the values of the angles $\alpha_i$ converge.

These equations offer an exact solution, yet such a complex angular frequency chirp is practically challenging in realistic experimental conditions. For sufficient time window however, the angle time dependencies can be linearized ($\alpha_i \propto \xi_i$) and we can obtain an analytical formula.

### B. Angle linearization approach

By employing a pair of prisms and a focusing element it is feasible to obtain an approximately linear angular chirp, provided that the quadratic distortion of the optical elements can be considered negligible. We can thus search for the analytical expression for the angles in the form

$$\alpha_i(\xi_i) = \alpha_{0,i} + \alpha_i^{'}\xi_i \tag{S9}$$

where $\alpha_{0,i}$ are the phase matching angles for frequencies $\omega_{0,i}$. The parameters $\alpha_i^{'}$ are considered constant. Under the assumption where $\alpha_i^{\prime}\xi_i$ is small, we approximate $\xi_i \approx \xi_i(\alpha_{0,i})$ and we assume we can use Taylor expansion to approximate trigonometric functions

$$sin(\alpha_{0,i} + \alpha_i^{'}\xi_i\ ) = sin(\alpha_{0,i}) + cos(\alpha_{0,i})\alpha_i^{'}\xi_i\ , \tag{S10}$$

$$cos(\alpha_{0,i} + \alpha_i^{'}\xi_i\ ) = cos(\alpha_{0,i}) - sin(\alpha_{0,i})\alpha_i^{'}\xi_i\ . \tag{S11}$$

Moreover, when the changes of the phase matching angles (S9) are assumed to be relatively small then the terms with higher order dependence on $\xi_i$ than linear can be neglected. Plugging Eq. (S9) into Eq. (S1) and using Eq. (S2) with the assumptions Eq. (S10), Eq. (S11) the following expression for $\alpha_1^{'}$ and $\alpha_2^{'}$ can be derived

$$\begin{pmatrix}\alpha_1^{'}\\ \alpha_2^{'}\end{pmatrix} = \frac{2}{\omega_{0,1}\omega_{0,2}sin(\alpha_{0,2}-\alpha_{0,1})}\begin{pmatrix} a_2\omega_{0,2} - a_1\omega_{0,2}sin(\alpha_{0,1}+\alpha_{0,2}) + \frac{c}{v_0}\omega_{0,2}(a_1-a_2)cos(\alpha_{0,2}) \\ -a_1\omega_{0,1} + a_2\omega_{0,1}sin(\alpha_{0,1}+\alpha_{0,2}) + \frac{c}{v_0}\omega_{0,1}(a_1-a_2)cos(\alpha_{0,1})\end{pmatrix} \tag{S12}$$

### C. Calculation of the phase matching angles

Now we directly calculate the required chirp of the optical fields, determined by the chirp that the electron pulse acquires after propagation in vacuum. Without loss of generality, we set $\mathbf{r}_{lab} = 0$. This allows us to use $t$ and $-z/v_0$ interchangeably. For $\mathbf{r}_{lab} = 0$ the optical pulse wave argument becomes $\xi = t = -z/v_0$.

The chirped electron pulse is described by the relationship between its instantaneous energy $E(z/v_0)$ and the corresponding rest frame coordinate which reads $E(z/v_0) = E_0 - \epsilon z/v_0$. We require that one of the created side-bands in the electron spectrum after the interaction with light has a constant energy with respect to the rest frame coordinate $z$, which leads to $E(z/v_0) + N\hbar\tilde{\omega}(z/v_0) = \text{const.}$, where $N$ denotes the number of the side-band. For example, the third and second harmonic frequency of the Nd:YAG can be used for the experiment. The angular frequencies are $\omega_{0,1} \doteq 5.47\ \text{fs}^{-1}$ and $\omega_{0,2} \doteq 3.65\ \text{fs}^{-1}$ corresponding to $\hbar\omega_{0,1} \doteq 3.6$ eV and $\hbar\omega_{0,2} \doteq 2.4$ eV . Then the chirps of the optical pulses are tied to the chirp of the electron pulse

$$E_0 - \epsilon z/v_0 + N\hbar(\omega_{0,1} - 2a_1 z/v_0 - \omega_{0,2} + 2a_2 z/v_0) = \text{const.}, \tag{S13}$$

which is true for $\epsilon = 2N\hbar(a_2 - a_1)$. For simplicity we chose $a_2 = -a_1$ and we limit ourselves to the first side-band $N = 1$.

For $\epsilon = \frac{0.5\,\text{eV}}{250\,\text{fs}}$, the required optical chirp is $a_{1,2} = \pm 7.6\cdot 10^{-4}\ \text{fs}^{-2}$. The approximate phase-matching angles of incidence are $\alpha_1 = 38.63\,^{\circ} + t\,0.058\,^{\circ}\text{fs}^{-1}$ and $\alpha_2 = 110.54\,^{\circ} - t\,0.086\,^{\circ}\text{fs}^{-1}$. The comparison between the exact and linearized dependence of $\alpha_1$ and $\alpha_2$ on time is shown in Fig. 2 in the main article. Even though the assumption that the change in $\alpha_i$ is small does not hold well, the linearly approximated angles closely follow the nonlinear numerical solution near the centre of the electron pulse. The validity of the phase matching angles is truly justified once the phase change is calculated.

## II. DESCRIPTION OF THE INTERACTION

### A. Interaction Hamiltonian

The Hamiltonian of the free electrons propagating in vacuum is $\hat{H}_0 = \hat{\mathbf{p}}^2/2m_e$, where $m_e$ is the electron mass and $\hat{\mathbf{p}}$ is the momentum operator. In the presence of an external field, the Hamiltonian becomes

$$\hat{H} = \frac{1}{2m}(\hat{\mathbf{p}} + e\mathbf{A})^2, \tag{S14}$$

where $e > 0$ is the elementary charge charge and $\mathbf{A}$ is the vector potential. The interaction part of the Hamiltonian can be separated into two components $\hat{H}_{\text{int}} = e(\mathbf{A}\cdot\hat{\mathbf{p}} + \hat{\mathbf{p}}\cdot\mathbf{A})/2m_e + e^2\mathbf{A}^2/2m_e$. We solve interaction between electrons and light in Dirac picture with respect to the free-evolution part. If the conditions are typical to those in electron microscopes, under an assumption that the energy spread of the electrons is relatively small compared to their mean energy $\Delta E/E_0 \approx 0$, the evolution of the system can be expressed in terms of the evolution operator, which reduces to a phase modulation [S2]

$$\hat{U} = \exp\left[-\frac{i}{\hbar}\int_{-\infty}^{\infty} H_{\text{int}}(\mathbf{r}_{\text{lab}}(t'), t')\,\text{d}t'\right]\ , \tag{S15}$$

where the Hamiltonian is evaluated along the classical trajectory of the electrons. Considering that the electrons propagate along the $z_{\text{lab}}$ direction with approximately constant group velocity $v_0$, we can treat the interaction as a 1D problem. We restate that it is convenient to evaluate the integral in the electron rest frame $z = z_{\text{lab}} - v_0 t$. The evolution operator then becomes

$$\hat{U}(z) = \exp\left[-\frac{i}{\hbar}\int_{-\infty}^{\infty} H_{\text{int}}(z,t')\,\mathrm{d}t'\right] , \tag{S16}$$

where $z$ is a parameter. The term $e(\mathbf{A}\cdot\hat{\mathbf{p}} + \hat{\mathbf{p}}\cdot\mathbf{A})/2m_e$ is important when the electrons interact with the optical modes of near-fields or semi-infinite fields, or in setups with significant light intensities. However, in vacuum for small intensities, this term becomes negligible, due to the velocity mismatch between the electron beam and the rapidly oscillating optical field. The leading term then becomes the ponderomotive scattering term $e^2\mathbf{A}^2/2m_e$ which accounts for the repulsion of electrons from areas with high light intensity to areas with low light intensity.

The total vector potential is given by the sum of the two vector potentials corresponding to the optical beams $\mathbf{A} = \mathbf{A}_1 + \mathbf{A}_2$. Under the assumption that fields are harmonic functions with slowly varying envelopes, $\mathbf{A}_i(t) \approx \mathbf{A}_{0,i}e^{-i\omega_i t}$, we can express the vector potential by an electric field $\mathbf{A}_i(t) = \mathbf{E}_i(t)/i\omega_i$. This relation is valid even for chirped optical pulses if the base frequency $\omega_{0,i}$ is substantially larger than the change in frequency acquired during the duration of the pulse because of the chirp $a_i$. The interaction Hamiltonian is explicitly:

$$H_{\text{int}} = \sum_{i,j=1}^{2}\frac{e^2}{2m}\mathbf{A}_i\cdot\mathbf{A}_j^* = -\sum_{i,j=1}^{2}\frac{e^2}{2m\omega_{0,i}\omega_{0,j}}\mathbf{E}_i\cdot\mathbf{E}_j^*. \tag{S17}$$

## B. Optical fields

To evaluate Eq. (S16) we need the explicit formulae for the optical fields $\mathbf{E}_i(\mathbf{r},t)$. In the first section we already established the spatio-temporally dependent frequencies $\omega_i(\xi_i)$ and angles $\alpha_i(\omega_i(\xi_i))$. Now we focus on formulating a suitable description of $\mathbf{E}_i(\mathbf{r},t)$.

The electric field of each of the optical beams with temporal and angular chirp (as established in Fig. S1) can be expressed as a sequence of quasi-monochromatic plane waves indexed by $j$ with temporal envelopes shifted in time to $\Delta_j$

$$\begin{aligned}\mathbf{E}_i(\mathbf{r},t) = \mathbf{e}_x\frac{E_{0,i}}{2}\sum_j\frac{\Delta_{j+1}-\Delta_j}{\sqrt{\pi}\sigma_{\text{coh}}}\exp\left(-\frac{\Delta_j^2}{\sigma_{\text{opt},i}^2}\right)\exp\left\{-\frac{\Big[\xi_i(\alpha_i(\Delta_j))-\Delta_j\Big]^2}{\sigma_{\text{coh}}^2}\right\}\times\\ \exp\left\{-\frac{x^2+[y\cos(\alpha_i(\Delta_j))-z\sin(\alpha_i(\Delta_j))]^2}{w_i^2}\right\}\exp\Big[-i(\omega_{0,i}+ia_i\Delta_j)\xi(\alpha_i)\Big]+\text{c.c.}.\end{aligned} \tag{S18}$$

The electric fields of both of the beams are polarized along the $\mathbf{e_x}$ direction, perpendicular to the plane drawn in Fig. S1. The peak amplitude of the electric field is $E_{0,i} = 2\cdot 10^9\ \text{V}\cdot\text{m}^{-1}$. The first exponential term is the amplitude of the quasi-monochromatic wave derived from the Gaussian shape of the chirped pulse. The parameter $\sigma_{\text{opt,i}}$ describes the duration of the entire optical pulse. The second term is the temporal envelope of that wave and it is delayed by its incidence time $\Delta_j$. The parameter $\sigma_{\text{coh}}$ describes the coherence time of the whole chirped optical pulse, which we model, and it is inversely proportional to the overall pulse spectral width. The third term describes a spatial modulation by Gaussian transverse envelope which is a reasonable approximation given the spatial overlap of the pulses being merely $9.94\ \mu$m which is much smaller than the Rayleigh lengths of the beams $54.9\ \mu$m and $228.8\ \mu\text{m}$. The fourth therm is the phase of wave.

In the previous section in Eqs. (S6)-(S8) or Eq. (S12) we show how to calculate the phase matching angles $\alpha_1(\xi_1)$ and $\alpha_2(\xi_2)$ explicitly. We note that the second exponential term localizes the spectral component around its corresponding time and position of arrival to the interaction region $\xi_i - \Delta_j$. By plugging $\xi_i = \Delta_j$ into Eq. (S5) and Eq. (S9), alternatively to Eq. (S5)-(S8), we obtain the instantaneous constant pulse frequency and constant angle of incidence for each spectral component by $\Delta_j$.

We transition to continuous $\Delta_j \to \Delta$, replace the summation with integration $\sum_j(\Delta_{j+1}-\Delta_j) \to \int d\Delta$. We consider the limit where the coherence time is much shorter than the pulse duration $\sigma_{\text{coh}} \to 0$

$$\lim_{\sigma_{\text{coh}}\to 0}\frac{1}{\sqrt{\pi}\sigma_{\text{coh}}}\exp\left\{-\frac{\Big[\xi_i(\alpha_i(\Delta))-\Delta\Big]^2}{\sigma_{\text{coh}}^2}\right\} = \delta(\xi-\Delta). \tag{S19}$$

Then the chirped electric fields can be simplified to the form

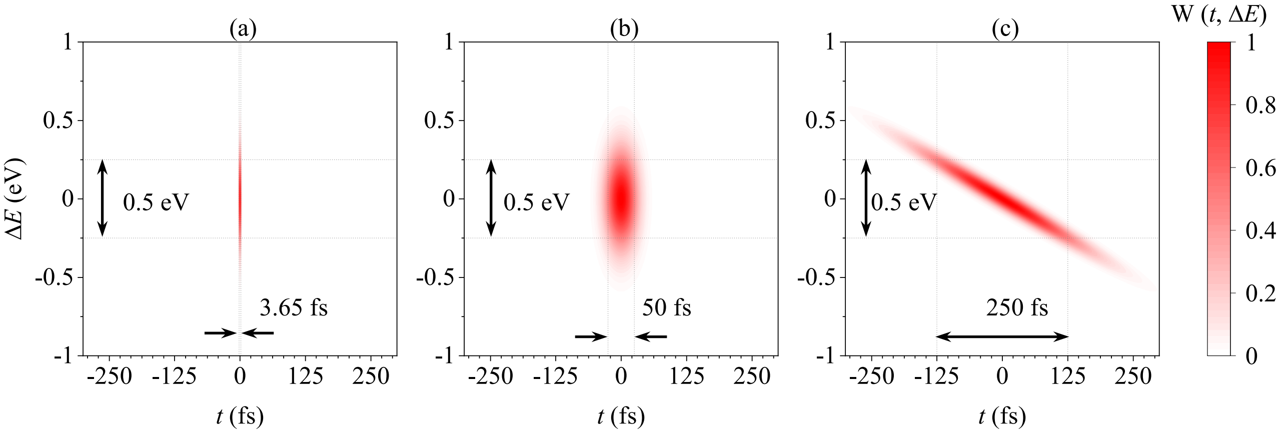


FIG. S2. Wigner function of the electron wave packet. (a) Representation of a fully coherent state with $\sigma_c = 2.19\,\mathrm{fs}$ (3.65 fs FWHM duration) and corresponding energy spread $\Delta E_{\mathrm{FWHM}} = 0.5\,\mathrm{eV}$. (b) The pulse is incoherently broadened with $\sqrt{\sigma_c^2 + \sigma_s^2} = 30\,\mathrm{fs}$ (50 fs FWHM duration), while the initial energy spread is perserved. (c) The pulse is elongated in time due to dispersive propagation in vacuum to $\sqrt{\sigma_c^2 + \sigma_s^2 + \sigma_p^2} = 150\,\mathrm{fs}$ (250 fs FWHM duration).

$$\mathbf{E}_i(\mathbf{r},t) = \mathbf{e}_x \frac{E_{0,i}}{2} \exp\left(-\frac{\xi^2(\alpha_i)}{\sigma_{\mathrm{opt},i}^2}\right) \times$$
$$\exp\left(-\frac{x^2 + (y\cos(\alpha_i) - z\sin(\alpha_i))^2}{w_i^2}\right) \exp\left(-i\omega_{0,i}\xi(\alpha_i) - i a_i \xi^2(\alpha_i)\right) + \mathrm{c.c.}. \tag{S20}$$

The polarization, the amplitude and the temporal envelope are in the first line of the equation while the transverse envelope and the chirped oscillations are expressed in the second line of the equation.

While the formula in Eq. (S18) relies on the discretization along the times of arrival of the spectral components of the pulse, the formula in Eq. (S20) describes a continuous wave with chirped frequency and also curved trajectory in space due to the angular chirp introduced by the pair of prisms and the lens. In the calculations we use Eq. (S20) as it eliminates the need for summing over a large number of spectral components. On the other hand, using the expression in Eq. (S18) can be advantageous, because the $\Delta_j$ parameter is an independent variable and the angles $\alpha_i$ are parameterized solely by $\Delta_j$ instead of $\xi_i$ which again depends on $\alpha_i$. Nevertheless, numerically both approaches yield equivalent results when the dicretization of Eq. (S18) is fine enough.

The parameters $w_1 = 5\ \mu\mathrm{m}$ and $w_2 = 3\ \mu\mathrm{m}$ stand for the waist $e^{-2}$ radii of the Gaussian spatial envelope. Given the geometry (Fig. S1) we chose such radii to achieve the optimal broadest phase matching along $z$ axis. Both beams have the same pulse duration of 250 fs full width at half maximum (FWHM), which is described by $\sigma_{\mathrm{opt},i} = 250/\sqrt{2ln(2)}$ fs. Given the parameters and a laser repetition frequency of 50 kHz the average powers of the beam are $P_1 = 2.77$ mW and $P_2 = 1$ mW. In practise two orders of magnitude higher average powers are easily achievable in table top setup, but the typical focal spots tend to be $\approx 10\ \mu\mathrm{m}$, which in the end leads to similar magnitudes of $E_{0,i}$.

### C. Wigner Function

We represent the electron wave packet with its Wigner function in phase space, see Fig. S2. Considering the Dirac picture with respect to free-space propagation, we omit the rapid oscillations and work with the envelope only. While the calculations are done in the coordinate-momentum space, the results are shown in the experimentally attainable time-energy space, with the axes $t = -z/v_0$, $\Delta E = E - E_0 = p v_0$. The spectral width of emitted electrons $\Delta E_{FWHM} = 0.5$ eV corresponds to the coherence length of $\sigma_{\mathrm{c}} \doteq 2,632$ fs or FWHM duration 3.65 fs via Fourier transform. The Wigner function of the coherent electron pulse is

$$W_{\mathrm{coh}} = \exp\left[-\begin{pmatrix} z, & p \end{pmatrix} \cdot \begin{pmatrix} \frac{1}{v_0^2\sigma_{\mathrm{c}}^2} & 0 \\ 0 & \frac{v_0^2\sigma_{\mathrm{c}}^2}{\hbar^2} \end{pmatrix} \cdot \begin{pmatrix} z \\ p \end{pmatrix}\right]. \tag{S21}$$

However, photoemission of electrons by a short ultraviolet pulse does not produce a fully temporally coherent electron wave packet but rather a wave packet with coherence time significantly shorter than the pulse duration. To describe such pulse we convolve the Wigner function of the coherent wave packet $W_{\rm coh}$ with a Gaussian smearing function $M$

$$M = \exp\left[-\begin{pmatrix} z, & p \end{pmatrix} \cdot \begin{pmatrix} \frac{1}{v_0^2\sigma_{\rm s}^2} & 0 \\ 0 & \delta \end{pmatrix} \cdot \begin{pmatrix} z \\ p \end{pmatrix}\right]. \tag{S22}$$

Afterwards we calculate the electron distribution before the interaction with the light fields using the convolution $W_{\rm inc} = \lim_{\delta\to 0} W_{\rm c} * M$. At the moment of emission from the tip the typical ultrashort incoherent electron pulse has length of 50 fs FWHM, which determines the $\sigma_{\rm s}$ parameter as $50^2/4ln(2) = \sigma_{\rm c}^2 + \sigma_{\rm s}^2$. This leads to following broadening in the direction of time in phase space, see Fig. S2 (b):

$$W_{\rm inc} = \exp\left[-\begin{pmatrix} z, & p \end{pmatrix} \cdot \begin{pmatrix} \frac{1}{v_0^2(\sigma_{\rm c}^2+\sigma_{\rm s}^2)} & 0 \\ 0 & \frac{v_0^2\sigma_{\rm c}^2}{\hbar^2} \end{pmatrix} \cdot \begin{pmatrix} z \\ p \end{pmatrix}\right]. \tag{S23}$$

Nonetheless as the pulse with finite $\Delta E$ propagates it acquires approximately a linear chirp due to dispersion in vacuum. The distribution in phase space must preserve its volume and its spectral width $\Delta E$. The pulse elongates to length 250 fs FWHM, which we have described by parameter $\sigma_{\rm p}$ given by $250^2/4ln(2) = \sigma_{\rm c}^2 + \sigma_{\rm p}^2 + \sigma_{\rm s}^2$. From these mathematical constrains we derive the following form of the Wigner function, see Fig. S2 (c):

$$W_{\rm in} = \exp\left[-\frac{1}{\hbar^2 v_0^2(\sigma_{\rm c}^2+\sigma_{\rm s}^2)}\begin{pmatrix} z, & p \end{pmatrix} \cdot \begin{pmatrix} \hbar^2 & -\hbar v_0^2\sigma_p\sigma_c \\ -\hbar v_0^2\sigma_{\rm p}\sigma_{\rm c} & v_0^4\sigma_{\rm c}^2(\sigma_{\rm c}^2+\sigma_{\rm p}^2+\sigma_{\rm s}^2) \end{pmatrix} \cdot \begin{pmatrix} z \\ p \end{pmatrix}\right]. \tag{S24}$$

The Wigner function can be transformed to the density matrix operator and vice versa trough a Wigner–Weyl transform:

$$\langle z|\hat{\rho}|z'\rangle = \int_{-\infty}^{\infty} \frac{dp}{\hbar} \exp\left[\frac{ip(z-z')}{\hbar}\right] W\left(\frac{z+z'}{2}, p\right) \tag{S25}$$

$$W(z,p) = \int_{-\infty}^{\infty} \frac{dy}{\pi\hbar} \exp\left[\frac{i2py}{\hbar}\right] \langle z-y|\hat{\rho}|z+y\rangle \tag{S26}$$

For the statistically broadened wave packet the density matrix operator cannot be separated into a dyadic product of wave functions. The analytical expression for the density matrix of the statistically broadened chirped pulse before interaction is:

$$\begin{aligned} \langle z|\hat{\rho}_{\rm in}|z'\rangle = \exp\Big[-\frac{(z+z')^2}{4v_0^2(\sigma_c^2+\sigma_s^2)}\Big]\times \\ \exp\left\{\frac{1}{v_0^2\sigma_c^2(\sigma_c^2+\sigma_s^2+\sigma_p^2)}\Big[\sigma_p\sigma_c\frac{z+z'}{2} + i(\sigma_c^2+\sigma_s^2)\frac{z-z'}{2}\Big]^2\right\} \end{aligned} \tag{S27}$$

We calculate the result of the light-electron interaction numerically through applying the evolution operator on the density matrix:

$$\langle z|\rho_{\rm out}|z'\rangle = \hat{U}(z)\langle z|\hat{\rho}_{\rm in}|z'\rangle\hat{U}^\dagger(z') \tag{S28}$$

Afterwards we transform $\rho_{out}$ back to Wigner function to get a representation in phase space, see Fig. S3 (a).

The Wigner distribution contains rapid oscillations on harmonic frequencies of the optical beat wave, which we explain in the next section. To better visualise the energetic state populations in Fig. S3(b) we used a spectrogram $S(z,p) = \lim_{\delta\to 0} W_{\rm out} * C$, where $C$ is:

$$C = \exp\left[-\begin{pmatrix} z, & p \end{pmatrix} \cdot \begin{pmatrix} \frac{1}{\Delta^2} & 0 \\ 0 & \delta \end{pmatrix} \cdot \begin{pmatrix} z \\ p \end{pmatrix}\right] \tag{S29}$$

The parameter of the averaging window was $\Delta \doteq 900$ nm. The spectrum $\langle p(E)|\hat{\rho}_{\rm out}|p(E)\rangle$ of the electron wave packet can be obtained from Wigner function:

$$\langle p(E)|\hat{\rho}_{\rm out}|p(E)\rangle = \int_{-\infty}^{\infty} W_{\rm out}(z,p)\, dz \tag{S30}$$

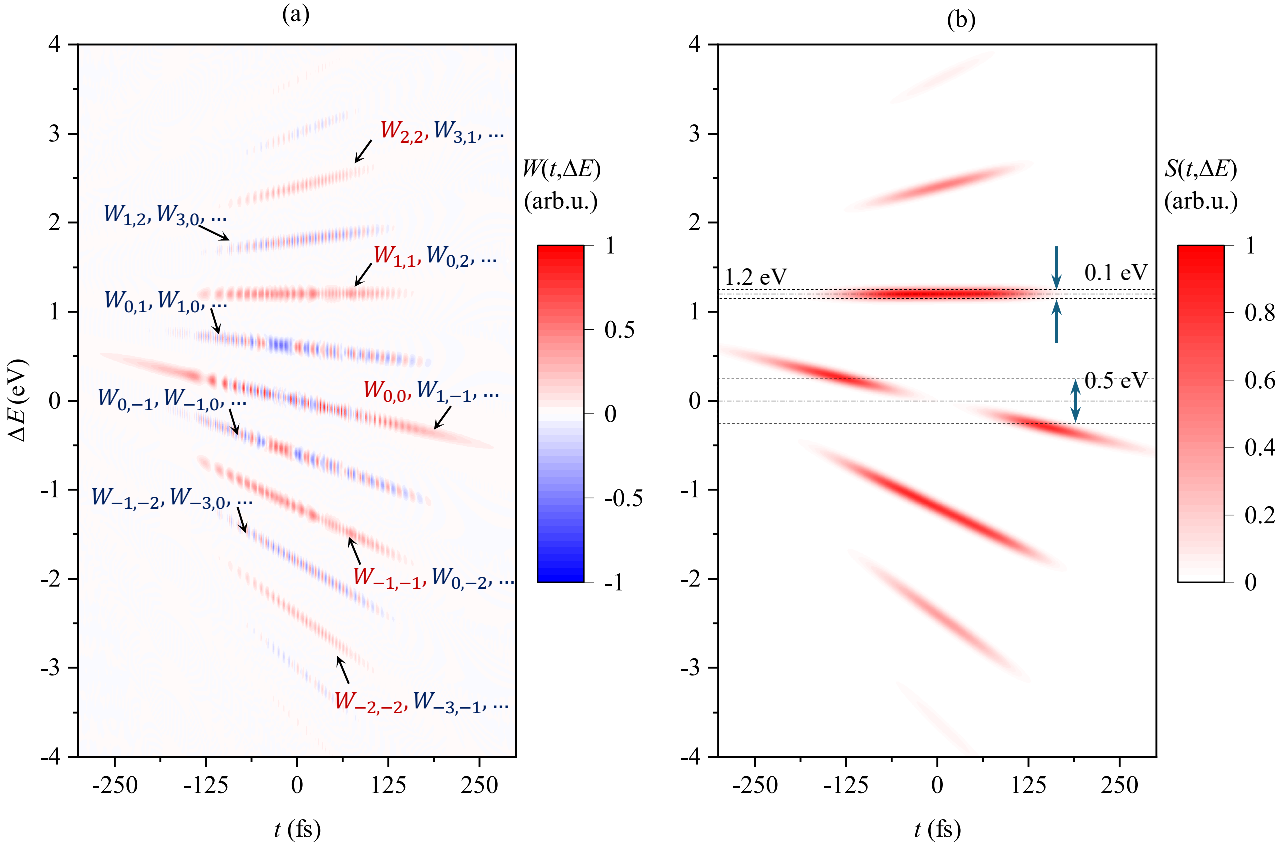


FIG. S3. (a) Wigner function of the electron wave packet after interaction with the chirped optical field. Between the energy side-bands representing real energy states separated by integer multiples of $\hbar\omega(t)$, oscillating coherences appear at half-integer multiples of $\hbar\omega(t)$. We assign the contributions to the Wigner function from the populations of the energy side-bands $W_{n,n}$ (red) and the coherences between the side-bands $W_{n,n'}$ (blue). (b) Spectrogram representing the real populations within the electron wave packet after interaction with the chirped optical field. From the initial $0.5\,\text{eV}$ wide original band, energy is transferred to the side-bands, with different tilts. The monochromatized first side-band is generated at $1.2\,\text{eV}$ with width of $0.1\,\text{eV}$.

## III. INTERPRETATION OF THE WIGNER FUNCTION OSCILLATIONS

In this section we introduce a simple model to explain the oscillatory behavior of the Wigner function of the electron wave packet after interaction with the optical beat wave. The electrons prior to the interaction are described by the density operator in the electron rest frame coordinate representation $\langle z|\hat{\rho}_{\text{in}}|z'\rangle$. For the sake of simplicity we now neglect the chirps of the optical pulses. Instead we consider the light grating to be created by two monochromatic optical pulses with constant difference frequency $\omega$. Then the evolution operator according to Eq. (S16) causes a simple sinusoidal phase modulation with constant frequency $\omega$, which in the electron rest frame takes the form:

$$\hat{U}(z) = \exp\left[-iA\sin\left(\frac{\omega}{v}z\right)\right], \tag{S31}$$

where the amplitude $A$ scales with the interaction strength and it is proportional to the square of the electric field amplitude for the case of ponderomotive scattering. For the evolution of the density matrix we plug Eq. (S31) into Eq. (S28). When we consider the Jacobi-Anger expansion of the evolution operator $\hat{U}(z)$, the Wigner integral according to Eq. (S26) is explicitly:

$$W(z,p) = \int_{-\infty}^{\infty}\frac{dy}{\pi\hbar}\exp\left[\frac{i2py}{\hbar}\right]\langle z-y|\hat{\rho}_{\text{in}}|z+y\rangle\sum_{n=-\infty}^{\infty}J_n(A)\exp\left[in\frac{\omega}{v}(z-y)\right]\sum_{n'=-\infty}^{\infty}J_{n'}(A)\exp\left[-in'\frac{\omega}{v}(z+y)\right], \tag{S32}$$

where $n$, $n'$ are integer indices, $J_n$ is the $n-th$ Bessel function of the first kind. We exchange the order of summation and integration and rearrange the terms:

$$W(z,p) = \sum_{n,n'=-\infty}^{\infty} J_n(A) J_{n'}(A) W_{n,n'}. \tag{S33}$$

We note that the Wigner function is constructed by summing the contributions $W_{n,n'}(z,p)$, weighted with the corresponding amplitudes $J_n(A)$, $J_{n'}(A)$, where

$$W_{n,n'}(z,p) = \int_{-\infty}^{\infty} \frac{dy}{\pi\hbar} \exp\left[\frac{i2py}{\hbar}\right] \langle z-y|\hat{\rho}_{\text{in}}|z+y\rangle \exp\left[i\frac{\omega}{v}\Big(n(z-y) - n'(z+y)\Big)\right]. \tag{S34}$$

We can interpret $W_{n,n'}(z,p)$ as the mixing of the $n$-th and $n'$-th side-band stemming from the bra- and ket- side of the density matrix.

Let us further consider weak interaction, where $A$ is such, that for $n > 1$ the amplitude $J_n(A)$ is negligible. Thus we need to take into account only the mixing between the zero-loss band and the first positive and negative side-bands. For example, $W_{0,0}(z,p)$ yields just the original zeroth band in the Wigner distribution before the interaction.

$$W_{0,0}(z,p) = \int_{-\infty}^{\infty} \frac{dy}{\pi\hbar} \exp\left[\frac{i2py}{\hbar}\right] \langle z-y|\hat{\rho}_{\text{in}}|z+y\rangle. \tag{S35}$$

In the cases $n = n' = \pm 1$, we obtain:

$$W_{\pm 1,\pm 1}(z,p) = \int_{-\infty}^{\infty} \frac{dy}{\pi\hbar} \exp\left[\frac{i2py}{\hbar}\right] \langle z-y|\hat{\rho}_{\text{in}}|z+y\rangle \exp\left[\mp i\frac{\omega}{v}2y\right], \tag{S36}$$

that results in the generation on the side-bands, that are copies of the original Wigner function shifted in the $p$ direction to $p' = p \mp \hbar\omega/v$. The case, where we consider the opposite side-bands $n = -n' = \pm 1$, we obtain:

$$W_{\pm 1,\mp 1}(z,p) = \exp\left[\pm i\frac{\omega}{v}2z\right] \int_{-\infty}^{\infty} \frac{dy}{\pi\hbar} \exp\left[\frac{i2py}{\hbar}\right] \langle z-y|\hat{\rho}_{\text{in}}|z+y\rangle, \tag{S37}$$

which is the zero-loss band, modulated by a factor oscillating at the second harmonic of the frequency of the optical grating. For mixing of $n = \pm 1$ and $n' = 0$ we obtain the contributions

$$W_{\pm 1,0}(z,p) = \exp\left[\pm i\frac{\omega}{v}z\right] \int_{-\infty}^{\infty} \frac{dy}{\pi\hbar} \exp\left[\frac{i2py}{\hbar}\right] \langle z-y|\hat{\rho}_{\text{in}}|z+y\rangle \exp\left[\mp i\frac{\omega}{v}y\right], \tag{S38}$$

which are shifted from the central band to $p' = p \mp \frac{1}{2}\hbar\omega/v$ and oscillate at the frequency of the optical grating $\omega$. The combination $n = 0$ and $n' = \mp 1$ yields the same contribution. This results in the generation of an oscillating band in between the two energy states, which can be interpreted as the coherence between the states.

This approach considers an optical grating with constant modulation frequency $\omega$ of the optical grid, which is sufficient to explain the oscillatory behavior. However a generalization to chirped grating with $\omega(z)$ is straightforward. In general, the cases where $n = n'$ describe the contributions from the populations of the side-bands and the cases where $n \neq n'$ describe the coherences between the side-bands. Introducing the mixing of all combinations of $n$ and $n'$ with nonzero amplitudes $J_{n,n'}(A)$ into the sum explains the more complicated features of the Wigner function with more energy states, like contributions of higher harmonic components in the oscillations.

While the incoherent broadening of the Wigner function described in Eq. (S24) occurs due to the uncertainty in the time of the photo-emission of the electron wave packet, the oscillations are purely an effect of the subsequent electron-light interaction, therefore they are expected even in incoherently broadened states.

[S1] M. Kozák, T. Eckstein, N. Schönenberger, and P. Hommelhoff, Inelastic ponderomotive scattering of electrons at a high-intensity optical travelling wave in vacuum, Nature Physics **14**, 121 (2018).

[S2] F. J. García de Abajo and A. Konečná, Optical modulation of electron beams in free space, Phys. Rev. Lett. **126**, 123901 (2021).
